# Supplementary material for: Understanding Android Obfuscation Techniques: A Large-Scale Investigation in the Wild
Source: arXiv:1801.01633 source file (2018-01-05)
Supplement: Supplementary file 1 [file appendix.tex]

\section{Appendix}
\label{appendix}

\subsection{Excessive Overloading Detection - Sample}
\label{appendix: overloading}
{\small
	\begin{lstlisting}[
	language={Java},
	label={lst:xxx},
	keywordstyle=\color{blue!70},
	numbers=left,                    
	numbersep=5pt, 
	xleftmargin=8pt,
	xrightmargin=5pt,
	numberstyle=\scriptsize\color{gray},
	breaklines=true,
	frame=single,
	%frame=shadowbox,
	basicstyle=\ttfamily,
	commentstyle=\color{blue} \textit,
	stringstyle=\ttfamily,
	showstringspaces=false]
public MD5State(){
  this.state = new int[2];
  this.state[0] = 1732584193;
  this.state[1] = -271733879;
}
//Signature: B[P1F1F0F0R]
	
public MD5State(MD5State from){
  int i;
  this.state = new int[2];
  for (i=0; i<this.state.length; i++){
    this.state[i] = from.state[i];
  }
}
//Signature: B[P1F1]B[F0I]B[F0F0G]B[R]
	\end{lstlisting} 
}

\ignore{
\subsection{Time-line based Study - Sample}
\label{appendix: time-line}

	\begin{lstlisting}[
	language={Java},
    label={lst:xxx},
	keywordstyle=\color{blue!70},
	numbers=left,                    
numbersep=5pt, 
xleftmargin=8pt,
xrightmargin=5pt,
numberstyle=\scriptsize\color{gray},
	breaklines=true,
	frame=single,
	%frame=shadowbox,
	basicstyle=\ttfamily,
	commentstyle=\color{blue} \textit,
	stringstyle=\ttfamily,
	showstringspaces=false]
public void onShutterButtonFocus(boolean pressed) { // version 4.0.1
  if (!this.mPausing && this.mCameraState != 3) {
    if (pressed && !canTakePicture()) {
      return;
    }
    if (pressed) {
      this.mFocusManager.onShutterDown();
    } else {
      this.mFocusManager.onShutterUp();
    }
  }
}
	\end{lstlisting}

	\begin{lstlisting}[
	language={Java},
    label={lst:xxx},
	keywordstyle=\color{blue!70},
	numbers=left,                    
numbersep=5pt, 
xleftmargin=8pt,
xrightmargin=5pt,
numberstyle=\scriptsize\color{gray},
	breaklines=true,
	frame=single,
	%frame=shadowbox,
	basicstyle=\ttfamily,
	commentstyle=\color{blue} \textit,
	stringstyle=\ttfamily,
	showstringspaces=false]
public void a(boolean z) { // version 5.0.1
  if (!this.aD && this.aF != 3) {
    if (z && !ap()) {
      return;
    }
    if (z) {
      this.ao.a();
    } else {
      this.ao.b();
    }
  }
}
	\end{lstlisting} 
}
